# Supplementary material for: Learning in brain-computer interface control evidenced by joint decomposition of brain and behavior
Source: arXiv:1908.00077 ancillary file (2019-08-02)
Supplement: Supplementary file 1 [file supp_v5.pdf]

# Supplementary Materials for
# "Learning in brain-computer interface control evidenced by joint decomposition of brain and behavior"

Jennifer Stiso[1,2], Marie-Constance Corsi[3,4], Jean M. Vettel[5,2,6], Javier Garcia[5,2], Fabio Pasqualetti[7], Fabrizio De Vico Fallani[3,4], Timothy H. Lucas[9], and Danielle S. Bassett[2,8,9,10,11,12,13]

[1] *Neuroscience Graduate Group, Perelman School of Medicine, University of Pennsylvania, Philadelphia, PA 19104, USA*

[2] *Department of Bioengineering, School of Engineering & Applied Science, University of Pennsylvania, Philadelphia, PA 19104, USA*

[3] *Inria Paris, Aramis project-team, F-75013, Paris, France*

[4] *Institut du Cerveau et de la Moelle Epinire, ICM, Inserm, U 1127, CNRS, UMR 7225, Sorbonne Universit, F-75013, Paris, France*

[5] *Human Research & Engineering Directorate, US CCDC Army Research Laboratory, Aberdeen, MD, USA*

[6] *Department of Psychological & Brain Sciences, University of California, Santa Barbara, CA, USA*

[7] *Department of Mechanical Engineering, University of California, Riverside, CA 92521*

[8] *Department of Electrical & Systems Engineering, School of Engineering & Applied Science, University of Pennsylvania, Philadelphia, PA 19104, USA*

[9] *Department of Neurology, Perelman School of Medicine, University of Pennsylvania, Philadelphia, PA 19104, USA*

[1]0*Department of Psychiatry, Perelman School of Medicine, University of Pennsylvania, Philadelphia, PA 19104, USA*

[11] *Department of Physics & Astronomy, College of Arts & Sciences, University of Pennsylvania, Philadelphia, PA 19104, USA*

[12] *The Santa Fe Institute, Santa Fe, NM 87501, USA and*

[13] *To whom correspondence should be addressed: dsb@seas.upenn.edu*

## SUPPLEMENTAL METHODS

### Optimal Control

In the methods section of the main text, we describe the notion of optimal control trajectories in rather broad strokes. Here in the supplement, we provide a more formal description. We begin by noting that from the formulation in Eq (6) in the main text, we can see that the term $(\mathbf{x}_T - \mathbf{x}(t))^T(\mathbf{x}_T - \mathbf{x}(t))$ constrains the trajectories of a subset of nodes by preventing the system from traveling too far from the target state. We can also see that the term $\rho \mathbf{u}_\kappa(t)^T \mathbf{u}_\kappa$ constrains the amount of input used to reach the target state, which is a requirement dictated by the underlying biology including metabolic demands and tissue sensitivities.

To solve the minimization problem stated in Eq (6) in the main text, we follow the derivation from [1]. Specifically, in order to compute an optimal $\mathbf{u^*}$ that induces a transition from the initial state $\mathbf{x}(0)$ to the target state $\mathbf{x}(T)$, we define the Hamiltonian as

$$H(\mathbf{p}, \mathbf{x}, \mathbf{u}_\kappa, t) = (\mathbf{x_T} - \mathbf{x})^\mathbf{T}(\mathbf{x_T} - \mathbf{x}) + \rho \mathbf{u}_\kappa^\mathbf{T} \mathbf{u} + \mathbf{p}(\mathbf{A}\mathbf{x} + \mathbf{B}\mathbf{u}_\kappa). \tag{1}$$

According to the Pontryagin minimization principle, if $\mathbf{u}_\kappa^*$ is a solution with the optimal trajectory $\mathbf{x}^*$, then there exists a $\mathbf{p}^*$ such that

$$\begin{aligned}
\frac{\partial H}{\partial \mathbf{x}} =& -2(\mathbf{x}_T - \mathbf{x}^*) + \mathbf{A}^T \mathbf{p}^* = -\dot{\mathbf{p}}^*, \\
\frac{\partial H}{\partial \mathbf{p}} =& \mathbf{A}\mathbf{x}^* + \mathbf{B}\mathbf{u}_\kappa, \\
\frac{\partial H}{\partial \mathbf{u}_\kappa} =& 2\rho {\mathbf{u}^*}_\kappa + \mathbf{B}^T \mathbf{p}^* = 0.
\end{aligned}$$

From the equations above, we can derive that

$${\mathbf{u}^*}_\kappa = -\frac{1}{2\rho}\mathbf{B}^T \mathbf{p}^*, \tag{2}$$

$$\dot{\mathbf{x}}^* = \mathbf{A}\mathbf{x}^* - \frac{1}{2\rho}\mathbf{B}\mathbf{B}^T \mathbf{p}^*, \tag{3}$$

such that the only unknown is now $\mathbf{p}^*$. Next, we can reduce this to

$$\begin{bmatrix} \dot{\mathbf{x}}^* \\ \dot{\mathbf{p}}^* \end{bmatrix} = \begin{bmatrix} \mathbf{A} & \frac{1}{2\rho}\mathbf{B}\mathbf{B}^\mathbf{T} \\ -2 & -\mathbf{A}^\mathbf{T} \end{bmatrix} \begin{bmatrix} \mathbf{x}^* \\ \mathbf{p}^* \end{bmatrix} + \begin{bmatrix} 0 \\ 2 \end{bmatrix} \mathbf{x}_T. \tag{4}$$

Let us define

$$\begin{aligned}
\tilde{\mathbf{A}} &= \begin{bmatrix} \mathbf{A} & \frac{1}{2\rho}\mathbf{B}\mathbf{B}^\mathbf{T} \\ -2 & -\mathbf{A}^\mathbf{T} \end{bmatrix}, \\
\tilde{\mathbf{x}} &= \begin{bmatrix} \mathbf{x}^* \\ \mathbf{p}^* \end{bmatrix}, \\
\tilde{\mathbf{b}} &= \begin{bmatrix} 0 \\ 2 \end{bmatrix} \mathbf{x}_T,
\end{aligned}$$

so that Eq. (4) can be rewritten as

$$\dot{\tilde{\mathbf{x}}} = \tilde{\mathbf{A}}\tilde{\mathbf{x}} + \tilde{\mathbf{b}}, \tag{5}$$

which can be solved as

$$\tilde{\mathbf{x}}(t) = e^{\tilde{\mathbf{A}}t}\tilde{\mathbf{x}}(0) + \tilde{\mathbf{A}}^{-1}(e^{\tilde{\mathbf{A}}t}\mathbf{x}(0) - \mathbf{I})\tilde{\mathbf{b}}. \tag{6}$$

Let

$$\mathbf{c} = \tilde{\mathbf{A}}^{-1}(e^{\tilde{\mathbf{A}}t}\tilde{\mathbf{x}}(0) - \mathbf{I})\tilde{\mathbf{b}}, \tag{7}$$

and

$$e^{\tilde{\mathbf{A}}T} = \begin{bmatrix} \mathbf{E}_{11} & \mathbf{E}_{12} \\ \mathbf{E}_{21} & \mathbf{E}_{22} \end{bmatrix} . \tag{8}$$

Then, by fixing $t = T$, we can rewrite Eq. (5) as

$$\begin{bmatrix} \dot{\mathbf{x}}^*(T) \\ \dot{\mathbf{p}}^*(T) \end{bmatrix} = \begin{bmatrix} \mathbf{E}_{11} & \mathbf{E}_{12} \\ \mathbf{E}_{21} & \mathbf{E}_{22} \end{bmatrix} \begin{bmatrix} \dot{\mathbf{x}}^*(0) \\ \dot{\mathbf{p}}^*(0) \end{bmatrix} + \begin{bmatrix} \mathbf{c}_1 \\ \mathbf{c}_2 \end{bmatrix} . \tag{9}$$

From this expression we can obtain

$$\mathbf{x}^*(T) = \mathbf{E}_{11}\mathbf{x}^*(0) + \mathbf{E}_{12}\mathbf{p}^*(0) + \mathbf{c}_1. \tag{10}$$

As a known result in optimal control theory [2], $\mathbf{p}^*(T) = 0$. Therefore,

$$\mathbf{p}^*(T) = \mathbf{E}_{21}\mathbf{x}^*(0) + \mathbf{E}_{22}\mathbf{p}^* + \mathbf{c}_2 = 0. \tag{11}$$

We can now solve for $\mathbf{p}^*(0)$ as follows:

$$\mathbf{p}^*(0) = \begin{bmatrix} \mathbf{E}_{12} \\ \mathbf{E_{22}} \end{bmatrix}^+ \left( - \begin{bmatrix} \mathbf{E}_{11} \\ \mathbf{E}_{21} \end{bmatrix} \mathbf{x}^*(0) - \begin{bmatrix} \mathbf{c}_1 \\ \mathbf{c}_2 \end{bmatrix} + \begin{bmatrix} \mathbf{x}(T) \\ 0 \end{bmatrix} \right) , \tag{12}$$

where $[]^+$ indicates the Moore-Penrose pseudoinverse of a matrix. Now that we have obtained $\mathbf{p}^*(0)$, we can use it and $\mathbf{x}^*$ (or $\mathbf{x}(0)$) to solve for $\tilde{\mathbf{x}}$ via forward integration. To solve for $\mathbf{u}^*{}_\kappa$, we simply take $\mathbf{p}^*$ from our solution for $\tilde{\mathbf{x}}$ and solve Eq. (5).

### *Optimal Control Energy of the System*

To quantify differences in the ease of controlling the system to a certain target state, we calculated a single measure of total energy for node $i$, defined as follows:

$$E_{i\mathbf{x}_0\mathbf{x}_T} = \int_0^T \mathbf{u}_{i\mathbf{x}_0\mathbf{x}_T} \mathrm{d}t \ . \tag{13}$$

A single measure of energy for the entire system was calculated by summing over all nodes in the network.

### *Metric for Simulation Error*

Because optimal control is a computationally difficult problem, we also calculate the numerical error associated with each computation. The numerical error is calculated as

$$n_{\mathrm{err}} = \left|\left| \left( \begin{bmatrix} \mathbf{E}_{12} \\ \mathbf{E}_{22} \end{bmatrix} \mathbf{p}^* \right) + \left( \begin{bmatrix} \mathbf{E}_{11} \\ \mathbf{E}_{21} \end{bmatrix} \mathbf{x}^*(0) + \begin{bmatrix} \mathbf{c}_1 \\ \mathbf{c}_2 \end{bmatrix} - \begin{bmatrix} \mathbf{x}(T) \\ 0 \end{bmatrix} \right) \right|\right| . \tag{14}$$

We minimize this error metric when choosing values for the free parameters $\rho$ and $T$, as described in more detail below.

### *Parameter Selection*

Our optimal control framework has two free parameters: $\rho$, the relative importance of the input constraint over the distance constraint, and $T$, the control horizon, or the amount of time given for the system to reach the target. Intuitively, choosing a lower value of the parameter $\rho$ corresponds to relaxing the constraint on the minimal energy, leading to larger energies but smaller errors. The final parameter $T$ determines how quickly the system is required to reach the target state. At small values of $T$, the system is difficult to control, leading to large errors and high energy requirements. At moderately large values of $T$, the system has more time to reach the target state, and simulations

typically produce smaller errors. At very large values of $T$, it is difficult to calculate the matrix exponentials, and simulations typically produce large errors.

Because we lack direct biological data that would inform the choice of these parameter values, we explored a range of values for both parameters, and we chose values that minimized the numerical error of the simulation. For each parameter, we first calculated the error of the simulations for parameter values that were logarithmically spaced between $1 \times 10^{-4}$ and 1 for $\rho$ and between 0.01 and 1 for $T$. We then selected the parameters that produced minimal error. Specifically, the parameters selected were $T = 0.1$ and $\rho = 0.1$. For the purposes of reliability and reproducibility, we also report results for two different sets of parameters that also produced low error. The two additional sets used were $T = 0.2$ and $\rho = 0.01$, and $T = 0.07$, and $\rho = 1$.

## Model Validation

In this work, we sought to test the hypothesis that regularized subgraphs of co-varying functional connectivity are well suited to modulate certain patterns of connectivity by positing a model of how activity would spread across connections defined by those subgraphs. It is important to note that the functional connectivity we study here reflects statistical dependencies between regions rather than causal interactions. However, since the subgraphs are regularized and were selected to maximize sparsity, they could be interpreted as possible paths of influence that are only weakly modulated by redundant relationships. Here we therefore investigated the validity of using these regularized subgraphs in our theoretical model of activity spread.

We operationalized this investigation by considering three properties of these subgraphs that would be required in order for them to be suitable for use in the control theoretic model. First, we sought to demonstrate that the regularization imposed by NMF leads to subgraphs with fewer triangles than functional connectivity matrices obtained without regularization [3]. Second, our model assumes that brain activity, at least on short time scales, evolves linearly along the connections of the network. This assumption leads to the testable prediction that simulating state transitions using Eq. 5 in the main text would yield states that bear some resemblance to empirical states. Third and finally, we wish to validate our claim that each subgraph contributed to a different part of the observed changes in brain state, and that that contribution is larger when that subgraph's temporal expression is higher relative to the other subgraphs.

To test the first prediction – that regularized subgraphs will have fewer triangles than the original functional connectivity matrices – we calculate the fraction of possible triangles present in the subgraphs as well as the average weight of each triangle. The first metric is calculated from a binarized version of the subgraph, while the second metric is calculated from the weighted version of the subgraph. For each subject, we report average values of each metric over subgraphs. Since the original functional connectivity matrices (prior to decomposition with regularization) are fully weighted and fully connected, they contain the maximum number of possible triangles. In contrast, subgraphs have approximately 30% of the possible triangles (Fig. S1A). Moreover, we observed a drastic reduction in the weight of triangles in the subgraphs compared to that observed in the original functional connectivity matrices (Fig. S1B). Together, these two results indicate that the process of regularization enacted by NMF removes many of the redundant relationships present in functional connectivity matrices.

We now turn to our second prediction that simulating state transitions using Eq. 5 in the main text would yield states that bear some resemblance to empirical states. It is unreasonable to expect noise free, time invariant linear models to fully capture neural dynamics at this time scale. Instead, we would like to ask if the features of network topology we are interested in provide additional explanatory power than similarly simple models that do not contain these features. We operationalize this prediction in the specific context of our experiment by stating that the third highest performance loading subgraph and the lowest performance loading subgraph should explain some of the changes in brain *activity* according to the following model of dynamics:

$$\dot{x}(t) = \mathbf{A}x(t) + \mathbf{B}u(t) \ , \tag{15}$$

where $x$ is the brain state at each sensor, $\mathbf{A}$ is the subgraph that we wish to test, and $\mathbf{B}u$ represents input to the left motor region during the BCI task.

To test our prediction, we use the above equation to obtain simulated brain states for each trial $t$ where $x(0)$ is the brain state at trial $t-1$, and we compare those simulated states to the observed brain states. Consistent with prior work [4], we define a brain state as a vector of power estimates in each channel, and we obtain such states separately for each frequency band. More specifically, for each trial we use FieldTrip (http://www.fieldtriptoolbox.org/) to implement a multitaper Fourier transform (method = 'mtmfft') with half taper smoothing. We then log transform the calculated power spectra, and $z$-score across trials and within sessions to obtain a brain state for each trial. For each trial, we then simulate the above equation with either the third highest or lowest performance loading subgraph as $\mathbf{A}$, the same $\mathbf{B}$ that was used in the main text (ones at regions in the left motor cortex, and a constant, smaller

number at other regions), and $u(t) = 1$. The time in the simulation is defined in arbitrary units, and thus it is not clear which time point to select that would be comparable to the 3 s trial interval. Here, we select 1000 arbitrary time steps to ensure that the system's response has stabilized. Then we select the time point at which the simulated state is most similar to the empirical brain state, where state similarity is given by the Pearson's correlation coefficient between the simulated state and the observed state. This procedure provides a measure of the best possible prediction that our model is capable of generating. We then average maximum correlations across trials to obtain one correlation value per subject. To ensure that our results were dependent on the true network topology of the empirical subgraphs, we repeated the same process with randomized networks that preserve the edge weight distribution, number of nodes, and number of edges of the original networks. These random networks are obtained using the 'randmio_und.m' function with 1000 swaps per edge from the Brain Connectivity Toolbox [5]. For both the third highest (paired $t$-test $t = 4.49$, $p = 3.67\times^{10-4}$) and lowest (paired $t$-test $t = 4.84$, $p = 1.75\times^{10-4}$) performance loading subgraphs, correlations are significantly larger than those obtained from the null model. Together, these results indicate that simulating state transitions using Eq. 5 in the main text does indeed yield states that are statistically similar to empirical states, and that that similarity is greater than expected in appropriate random network null models.

Lastly, we wished to test the final prediction that each subgraph will contribute more to future brain states when its expression is relatively high. We performed simulations using the same model described above, but this time we used each subgraph individually. More specifically, for every subgraph $\mathbf{C_i}$, we simulate the dynamics

$$\dot{x}(t) = \mathbf{C_i}x(t) + \mathbf{B}u(t) \ . \tag{16}$$

Ultimately, this process gives us the predicted states for every subgraph and every trial $\bar{\mathbf{X}}$, an $N \times m \times t$ vector where $N$ is the number of nodes, $m$ is the number of subgraphs, and $t$ is the number of trials. We can then estimate the weight of each prediction on the true state by solving for $d$ in

$$\dot{x}(t) = \bar{\mathbf{X}}(t)d(t) \ , \tag{17}$$

where $d$ is a $1 \times m$ vector. We can then test the similarity of $d$ to the temporal expression obtained from the NMF algorithm. Specifically, we $z$-score both $d$ and $\mathbf{W}$ across subgraphs to scale the data, and then assess the correlation coefficient between $d_i$ and $\mathbf{W_i}$ for each subgraph $i \in m$. We then average the correlation values over subgraphs. Lastly, we compare the observed mean correlations to those obtained from comparing $d_i$ to $\mathbf{W_j}$, where $j$ is drawn randomly with replacement from $m$. We find that correlations for the empirical data are significantly greater than 0 (permutation test: $p = 0.038$), and significantly greater than correlations obtained from unmatched subgraphs (permutation test, $p = 0.022$) (Fig. S1D). Together, these results indicate that a subgraph will contribute more to future brain states when its expression is relatively high, consistent with our prediction.

Collectively, the validation of our three predictions provides empirical support for our use of NMF-derived subgraphs as adjacency matrices in the network control framework.

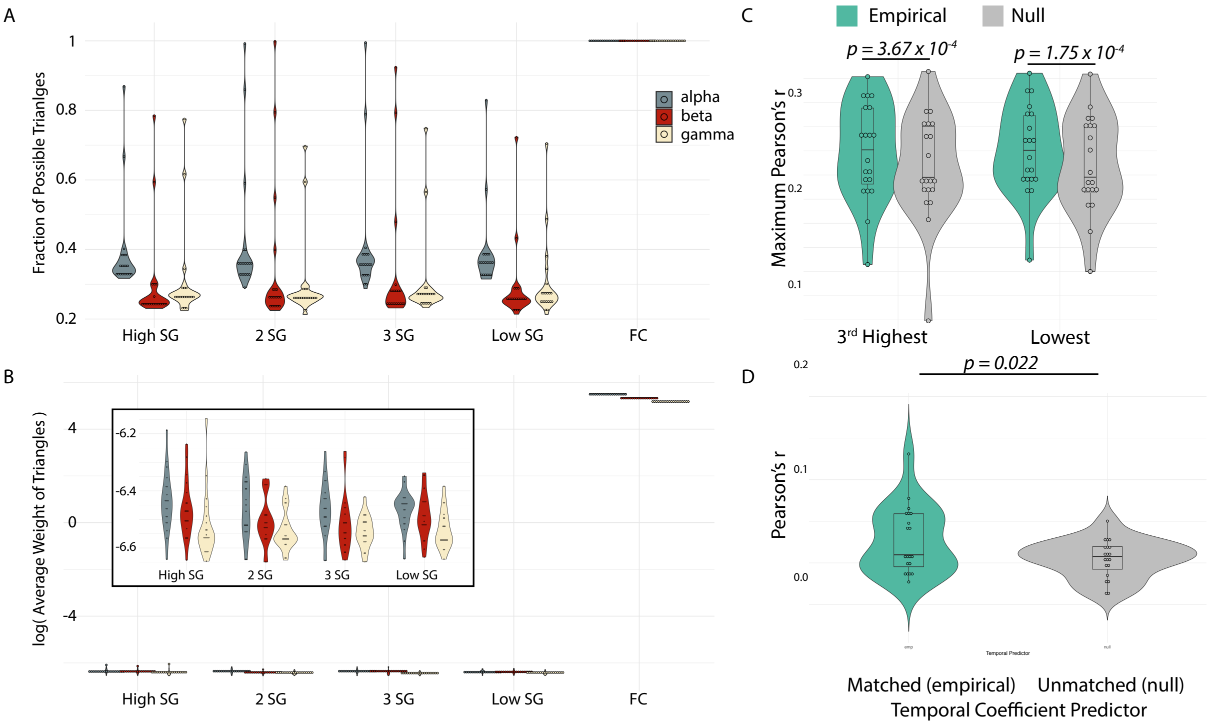


FIG. 1. **Effect of Regularization on Triangles.** (*A*) The fraction of present triangles over possible triangles in binarized graphs for each subgraph, and for the original functional connectivity (FC) matrices prior to NMF decomposition with regularization. (*B*) The average weight of triangles for each subgraph, and for the original FC matrices prior to NMF decomposition with regularization. The inset shows all subgraphs on a different scale. (*C*) Similarity between simulated and empirical brain states for third highest and lowest performance loading subgraphs. Each data point reflects the average of the maximum correlation reached over all trials ($N = 384$ if no trials were removed). Correlations from empirical subgraphs are shown in green, and correlations from randomized subgraphs are shown in grey. (*D*) The similarity between (i) the weighted contribution of each subgraph to predicting the next brain state and (ii) the temporal expression of that subgraph derived from NMF. Correlations from matched state prediction weights and temporal expression are shown in green, and correlations from mismatched temporal expression are shown in grey.

## SUPPLEMENTAL FIGURES

---

[1] S. Gu, R. F. Betzel, M. G. Mattar, M. Cieslak, P. R. Delio, S. T. Grafton, F. Pasqualetti, and D. S. Bassett, NeuroImage **148**, 305 (2017), arXiv:1607.01706.
[2] A. E. Bryson, IEEE Control Systems **16**, 26 (1996).
[3] A. Das, A. L. Sampson, C. Lainscsek, L. Muller, W. Lin, J. C. Doyle, S. S. Cash, E. Halgren, and T. J. Sejnowski, *Neural Computation*, Tech. Rep. 3 (2017) arXiv:1309.2848v1.
[4] J. Stiso, A. N. Khambhati, T. Menara, A. E. Kahn, J. M. Stein, S. R. Das, R. Gorniak, J. Tracy, B. Litt, K. A. Davis, F. Pasqualetti, T. Lucas, and D. S. Bassett, (2018), 10.1101/313304, arXiv:1805.01260.
[5] M. Rubinov and O. Sporns, NeuroImage **52**, 1059 (2010).

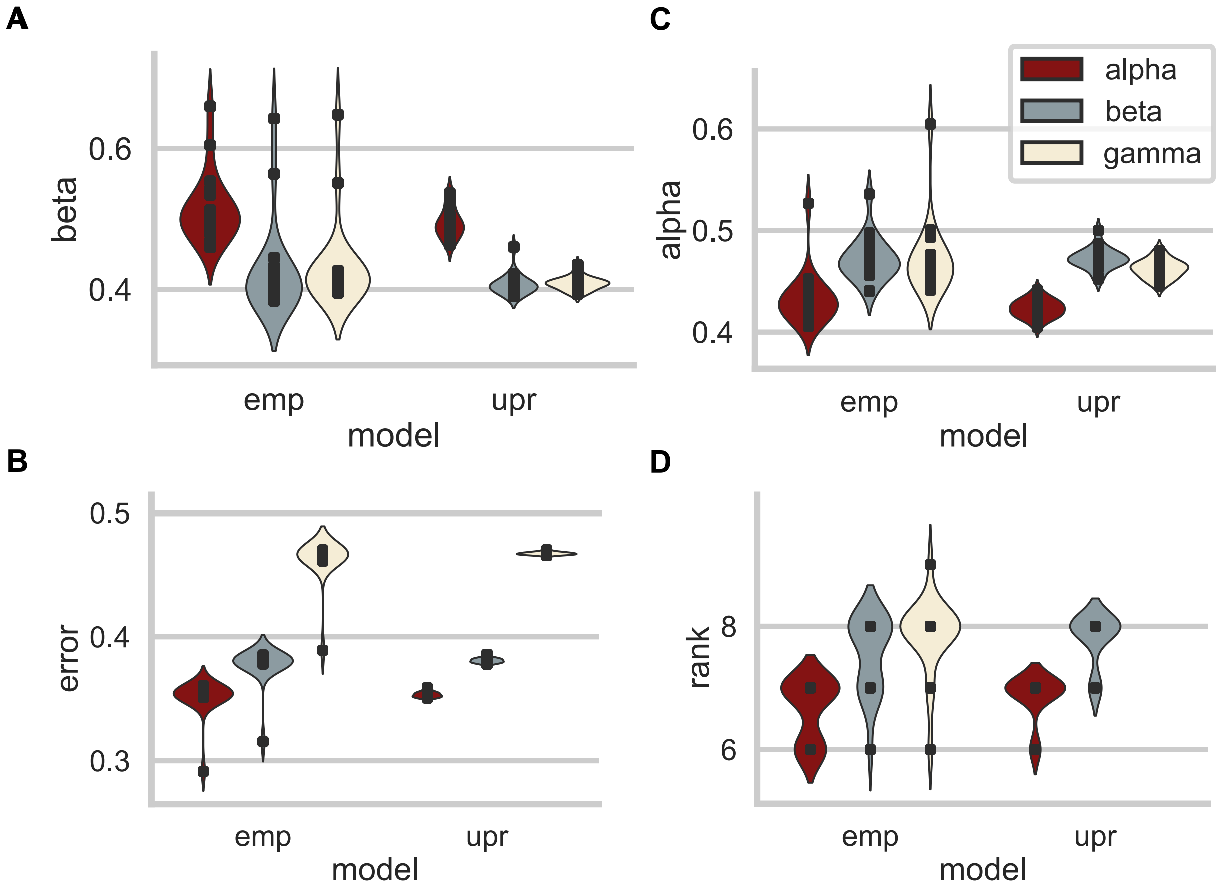


FIG. 2. **NMF Parameters.** Distributions of all three NMF parameters (panel $A$, $\beta$; panel $C$, $\alpha$; panel $D$, $m$) and error (panel $B$) for empirical data (*emp*) and null data (*upr*, indicating **u**niformly **p**hase **r**andomized null model). Each band is shown in a different color: $\alpha$ band (red), $\beta$ band (grey-blue), and $\gamma$ band (cream).

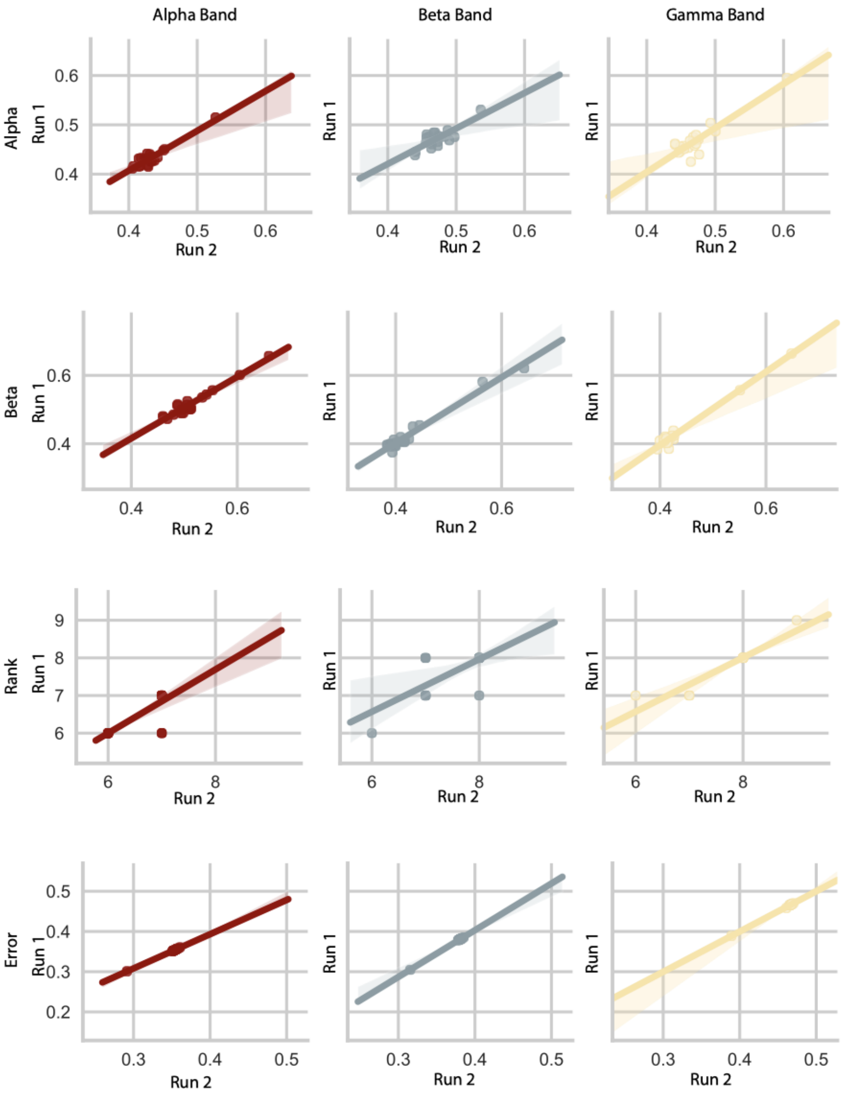


FIG. 3. **NMF Parameter Consistency.** The consistency of NMF parameters across two randomly chosen runs of the algorithm: run $i$ marked by the x-axis, and run $j$ marked by the y-axis. Each parameter is given in a different row: $\alpha$ (top row), $\beta$ (second row), rank (third row), and error (bottom row). Each band is shown in a different color: $\alpha$ band (red, left), $\beta$ band (grey-blue, middle), and $\gamma$ band (cream, right). Each data point indicates the selected parameter for a single subject.

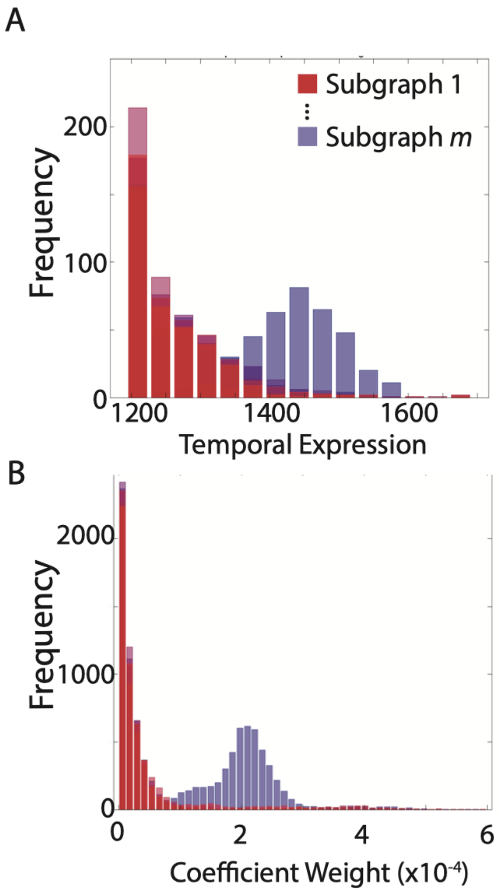


FIG. 4. **Mean Subgraphs.** Example histograms from a representative subject showing how one subgraph ($m$, shown in purple) has drastically different distributions of ($A$) temporal expression and ($B$) coefficients than the others. These outlier subgraphs were removed from further analysis to allow us to investigate differences among the remaining more local subgraphs. Different subgraphs are plotted in different colors.

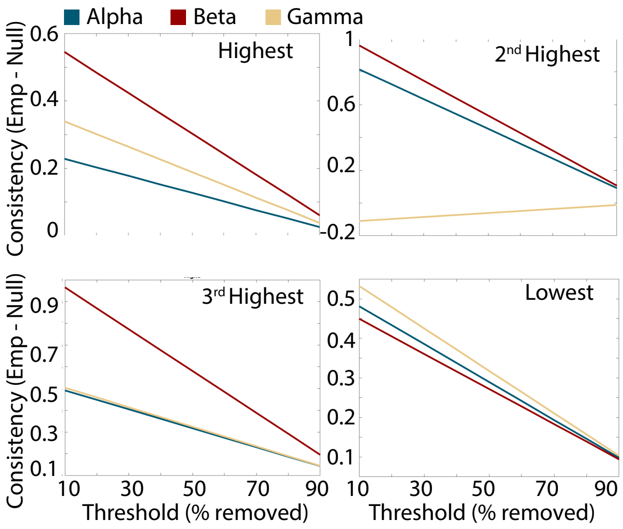


FIG. 5. **Consistency Across Thresholds.** To quantify spatial features common to each subgraph, we calculate the average consistency of each edge, or the number of subjects that had a given edge in their X% strongest connections. Here, we plot the difference in average consistency between empirical and null data changes with the choice of different thresholds (choices of X). Notice that for any choice of threshold, the relationship between null and empirical graphs for a given band has the same sign, and that generally null data is less consistent (except for the $\gamma$ band in the second highest subgraph). Each frequency band is shown in a different color: $\alpha$ band (red), $\beta$ band (grey-blue), and $\gamma$ band (cream). Results are shown for the highest performance loading subgraph (top left), second highest performance loading subgraph (top right), third highest performance loading subgraph (bottom left), and lowest performance loading subgraph (right).

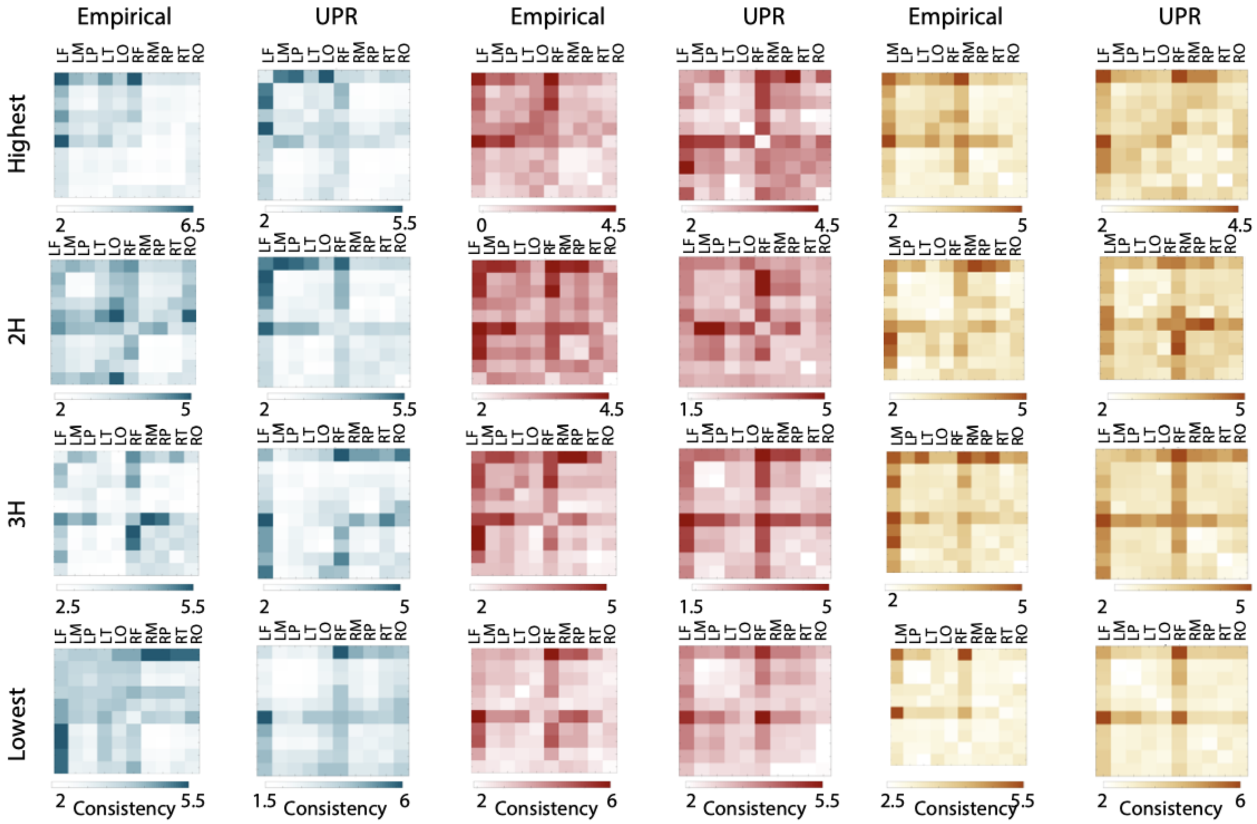


FIG. 6. **Consistency for Null Data.** The consistent subgraphs identified for the uniformly phase randomized null data (*UPR*) and for the empirical data (*Empirical*). Each frequency band is shown in a different color: $\alpha$ band (red, two leftmost columns), $\beta$ band (grey-blue, two middle columns), and $\gamma$ band (cream, two rightmost columns). The color bar reflects consistency, or the number of subjects that had a given edge in their 25% strongest connections.

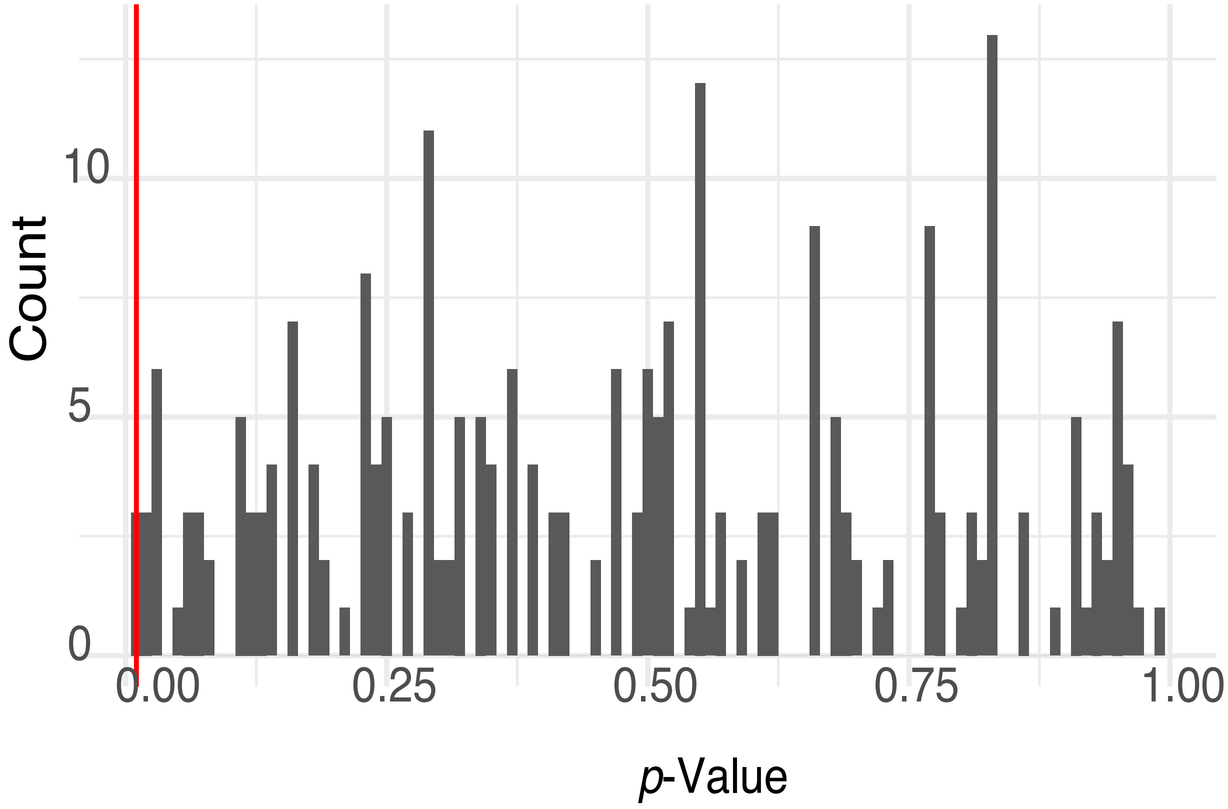


FIG. 7. **Alternate target states with the same magnitude.** A histogram of the correlation between the energy difference for low and third highest subgraphs to reach a spatially shifted brain state with the same magnitude as the attention state, and the learning rate for 500 randomly shifted target states. The red line indicates the observed $p$-value.

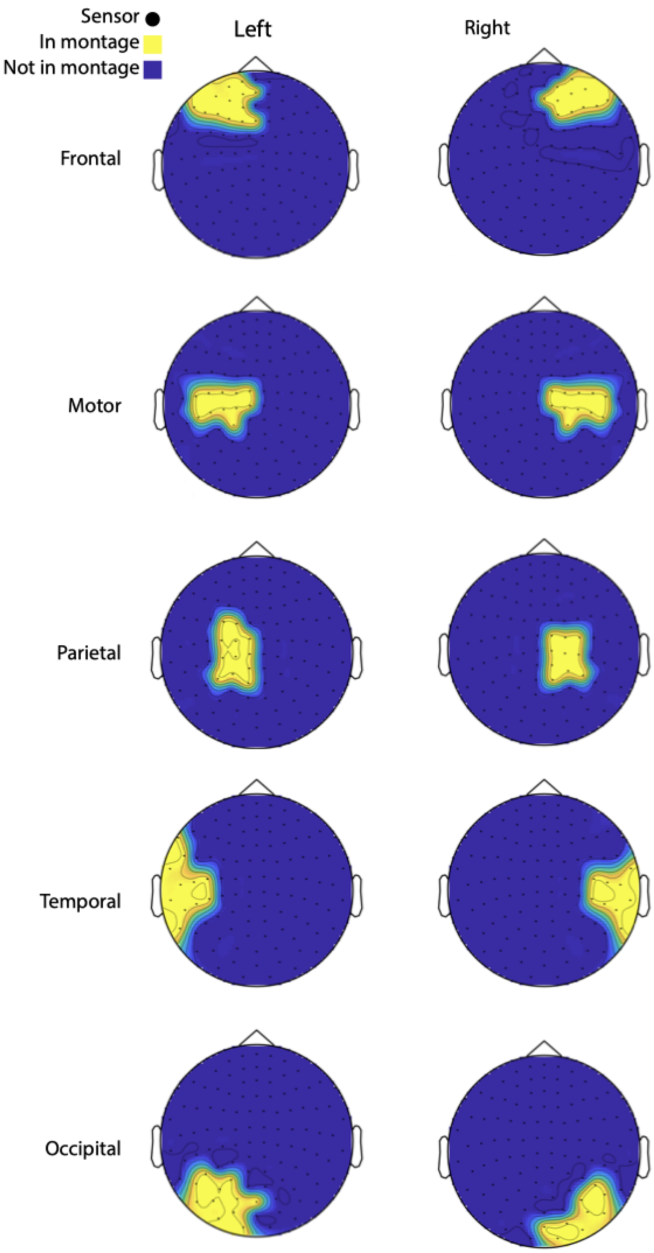


FIG. 8. **Montages.** Masks of the montages used to define regions for consistency analyses. Black dots indicate sensor locations. Yellow areas indicate regions included in the montage; dark blue areas indicate regions not included in the montage. Columns indicate hemisphere. Rows indicate lobe or swath: frontal (top), motor (second), parietal (third), temporal (fourth), and occipital (bottom).

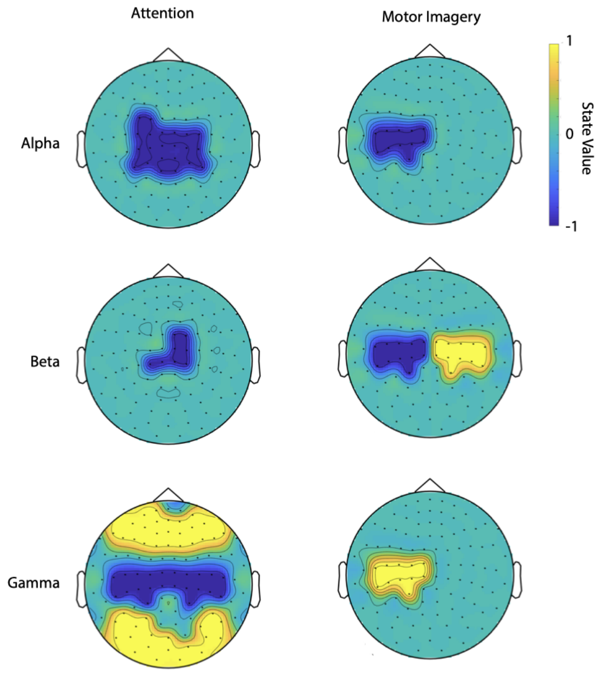


FIG. 9. **Optimal Control Target States.** Masks of the target states used for the optimal control analyses. Each state is a linear combination of the montages displayed in the previous figure. Color indicates state value. The left column shows the attention state for the $\alpha$ band (top), $\beta$ band (middle), and $\gamma$ band (bottom); the right column shows the motor state for the $\alpha$ band (top), $\beta$ band (middle), and $\gamma$ band (bottom).

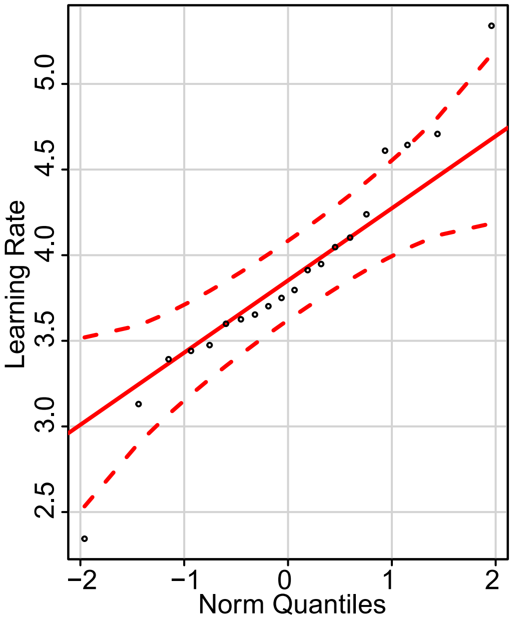


FIG. 10. **Normality of Performance.** Quantile-quantile plot for the performance in each session across subjects. Each data point indicates a subject. Most of the data points fall near the red line, indicating a normal distribution. Dotted red lines represent the 95% confidence interval.

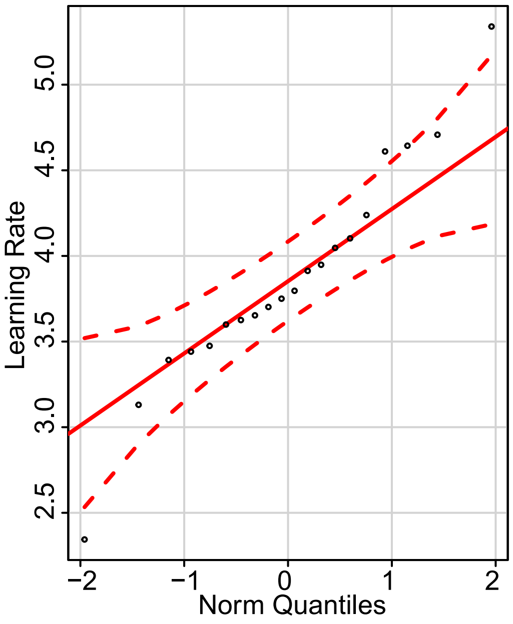


FIG. 11. **Normality of Learning Rate.** Quantile-quantile plot for the learning rate across subjects. Each data point indicates a subject. Most of the data points fall near the red line, indicating a normal distribution. Dotted red lines represent the 95% confidence interval.

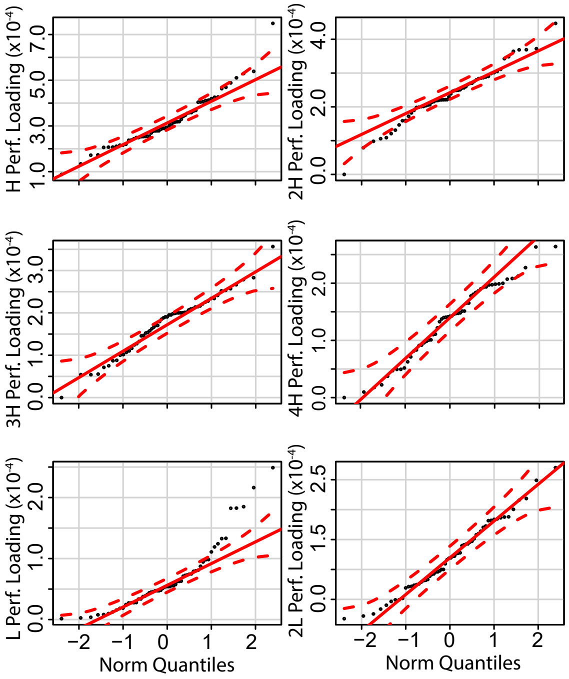


FIG. 12. **Normality of Performance Loading for Empirical Data.** Quantile-quantile plots for performance loading across subjects. Each data point indicates a subject and band. Each panel displays data from a different subgraph: the highest performance loading subgraphs (top left), the second highest performance loading subgraph (top right), the third highest performance loading subgraph (middle left), the fourth highest performance loading subgraph (middle right), the lowest performance loading subgraph (bottom left), and the second lowest performance loading subgraph (bottom right). Note that some of the data does not fall near the red line, indicating a non-normal distribution. In each panel, the dotted red lines represent the 95% confidence interval.

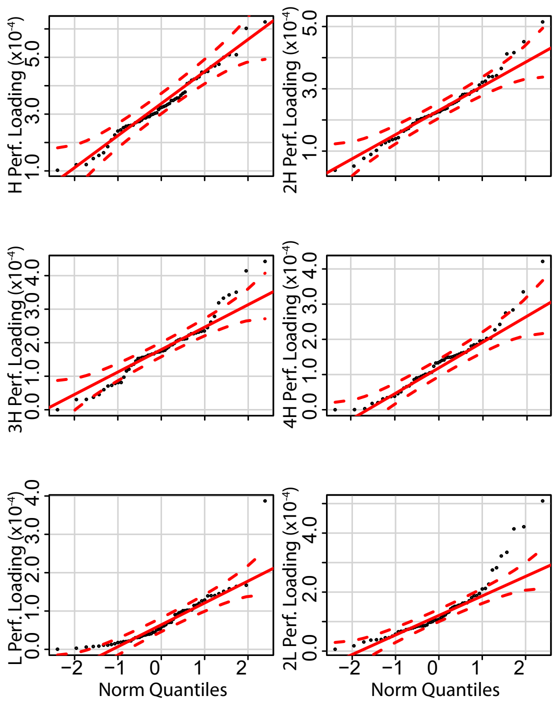


FIG. 13. **Normality of Performance Loading for Null Data.** Quantile-quantile plots for performance loading across subjects from the uniformly phase randomized null data. Each data point indicates a subject and band. Each panel displays data from a different subgraph: the highest performance loading subgraphs (top left), the second highest performance loading subgraph (top right), the third highest performance loading subgraph (middle left), the fourth highest performance loading subgraph (middle right), the lowest performance loading subgraph (bottom left), and the second lowest performance loading subgraph (bottom right). Note that some of the data does not fall near the red line, indicating a non-normal distribution. In each panel, the dotted red lines represent the 95% confidence interval.

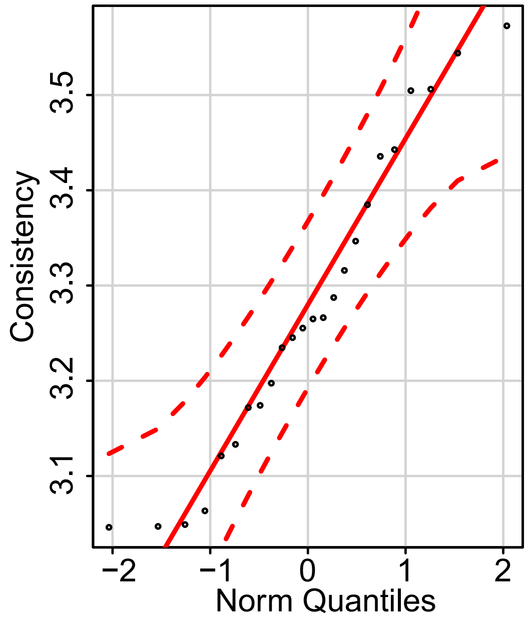


FIG. 14. **Normality of Consistency Data.** Quantile-quantile plot for the consistency across subjects. Each data point indicates a subject and band. Most of the data points fall near the red line, indicating a normal distribution. Dotted red lines represent the 95% confidence interval.

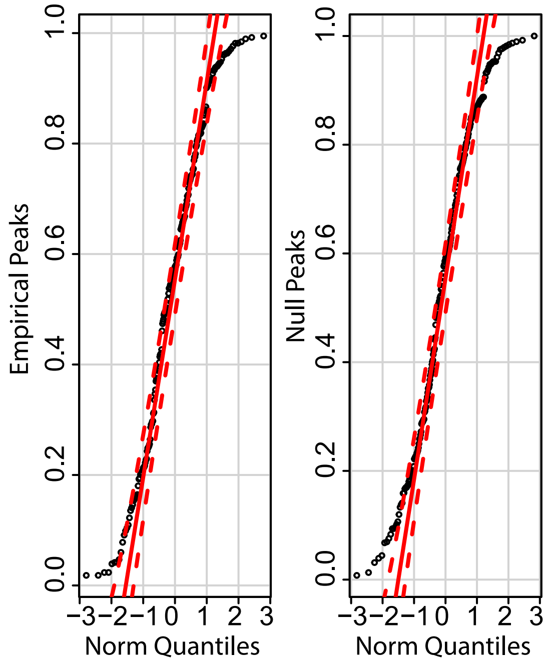


FIG. 15. **Normality of Peak Temporal Expression Data.** Quantile-quantile plots for the peak expression across subjects, bands, and subgraphs. Each data point indicates a subgraph for a given subject and band. Empirical data is shown on the left and uniformly phase randomized data is shown on the right. Most of the data points fall near the red line, indicating a normal distribution. Dotted red lines represent the 95% confidence interval.

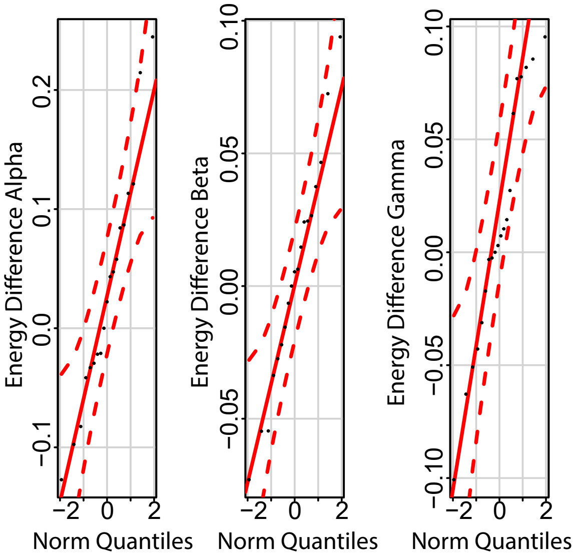


FIG. 16. **Normality of Energy Difference to Attention States.** Quantile-quantile plots for the optimal energy difference in attention states across subjects, separately for the $\alpha$ band (left), $\beta$ band (middle), and $\gamma$ band (right). Each data point indicates a subject. Most of the data points fall near the red line, indicating a normal distribution. Dotted red lines represent the 95% confidence interval.

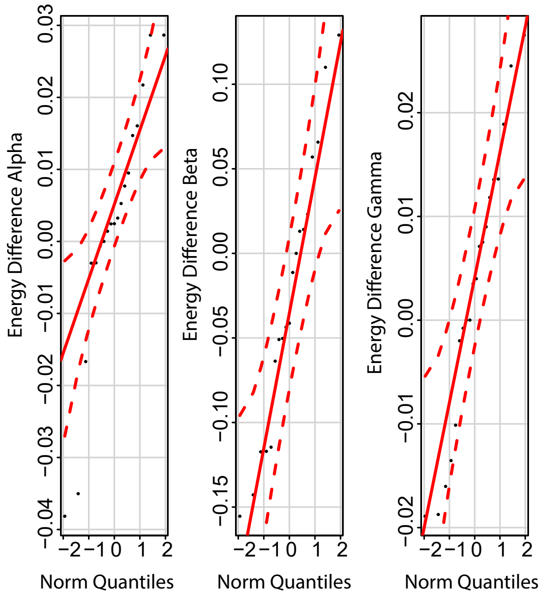


FIG. 17. **Normality of Energy Difference to Motor Imagery States.** Quantile-quantile plots for the optimal energy difference of motor imagery states across subjects, separately for the $\alpha$ band (left), $\beta$ band (middle), and $\gamma$ band (right). Each data point indicates a subject. Most of the data points fall near the red line, indicating a normal distribution. Dotted red lines represent the 95% confidence interval.

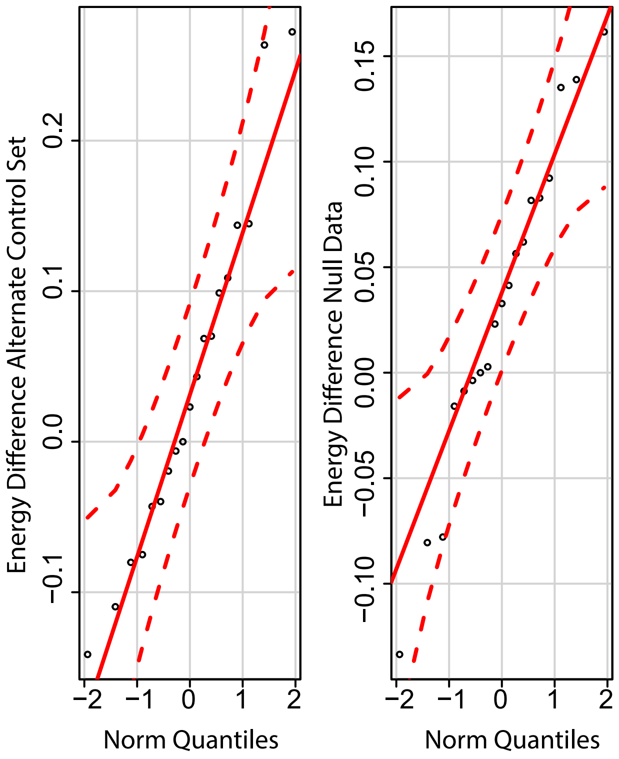


FIG. 18. **Normality of Energy Difference for Alternate Control Set and for Null Data.** Quantile-quantile plots for the optimal energy difference of null analyses across subjects. The left panel show data for the alternative control set and the right panel shows data for the uniformly phase randomized null. Each data point indicates a subject. Most of the data points fall near the red line, indicating a normal distribution. Dotted red lines represent the 95% confidence interval.

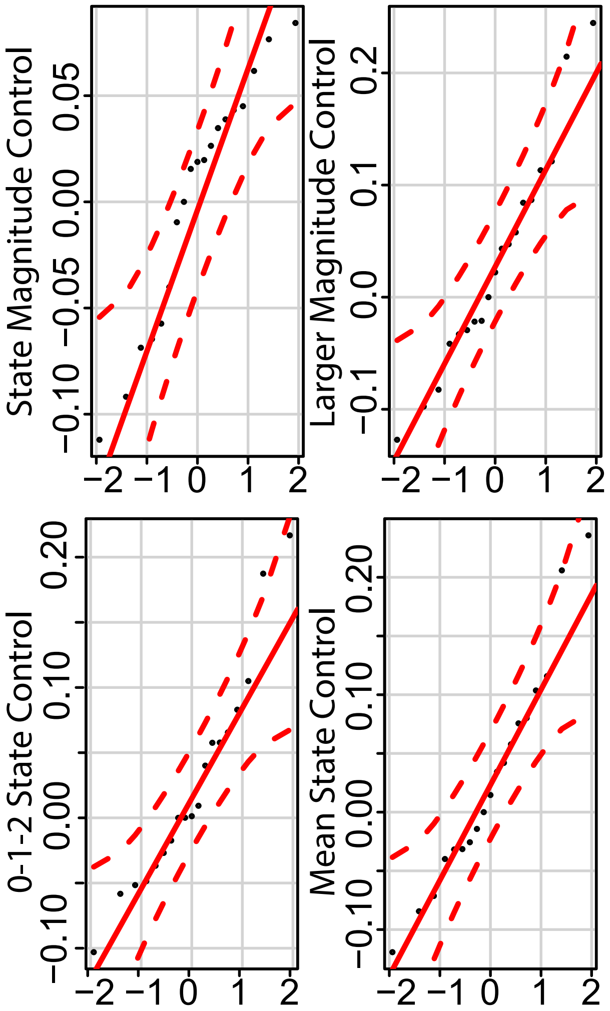


FIG. 19. **Normality of Energy Difference for Various State Controls.** Quantile-quantile plots for the optimal energy difference of state control analyses across subjects. These analyses include a control for state magnitude (top left), a control for larger magnitude (top right), a control changing the state intervals (bottom left), and a control for the mean state (bottom right). Each data point indicates a subject. Most of the data points fall near the red line, indicating a normal distribution. Dotted red lines represent the 95% confidence interval.
